# Supplementary material for: DoT: An efficient Double Transformer for NLP tasks with tables
Source: arXiv:2106.00479 source file (2021-06-01)
Supplement: Supplementary file 2 [file supplementary.tex]

\documentclass[11pt,a4paper]{article}
\input{style/preamble}
% \usepackage[1-6]{pagesel}
%\usepackage[7-]{pagesel}

%%%%%%%%%%%%%%%%%%%%%%%%%%%%%%%%%%%%%%%%%%%%%%%%%%%%%%%%%%%%%%%%%%%%%%%%

\myexternaldocument{main}

\begin{document}

\appendix
\latexfile{9-appendix}
% \bibliographystyle{style/acl_natbib}
% \bibliography{acl2020.bib}

\end{document}
